# Supplementary material for: Improved Nonnegativity Testing in the Bernstein Basis via Geometric Means
Source: arXiv:2309.10675 source file (2023-09-19)
Supplement: Supplementary file 1 [file P2Pproofs.tex]

\section{Proofs about properties of $\mathcal{GB}_n$}\label{sec:P2Pproofs}
We need to recall some basic facts about semidefinite matrices and the Hadamard product. First, we introduce some notation only used in this section. The symbol $\circ$ here refers to the Hadamard product. Let $\mathbf{1}_n$ be the $n \times n$ matrix of just 1's.

The following result is the Schur product theorem.

\begin{fact}\label{lem:kronproductpsd}
If $A, B \succeq 0$ then $A \circ B \succeq 0$.
\end{fact}
\begin{fact}\label{fact:2x2tonxn}
    If $\pmat{a & b \\ b & d} \succeq 0$, then $\pmat{a \mathbf{1}_n & b \mathbf{1}_n \\ b \mathbf{1}_n & d \mathbf{1}_n} \succeq 0$.
\end{fact}
\begin{proof}
We notice that $\pmat{a \mathbf{1}_n & b \mathbf{1}_n \\ b \mathbf{1}_n & d \mathbf{1}_n} = \pmat{a & b \\ b &d} \otimes \mathbf{1}_n$, and it is a well-known fact that the tensor product of two positive semidefinite matrices is positive semidefinite.
\end{proof}
\begin{lem}\label{lem:sumpsdblock}
If $\pmat{A & B \\ B^T  & D} \succeq 0 $ where $A, D \in S^n$ then $A + B+ B^T + D \succeq 0$. 
\end{lem}
\begin{proof}
Let $x \in \mathbb{R}^n$. Then $0 \leq \pmat{x \\ x}^T \pmat{A & B\\ B^T & D}\pmat{x \\ x} = x^T(A + B+ B^T + D)x$.
\end{proof}

This is enough to prove the second order cone analog of the scalar case.

\genmatrixnonnegativesocp*
\begin{proof}[Proof of Lemma~\ref{lem:gen_matrix_nonnegative_socp}.]
The matrix in the condition is congruent to
\begin{equation}\label{eqn:matrix_congruence_sufficient}
\pmat{\frac{w_{i-1}}{{m_i}}(P_{i-1}- C_{i-1} - C_{i-1}^T) & \sqrt{2}C_i \\ \sqrt{2}C_i^T & w_{i+1}(P_{i+1} - C_{i+1} - C_{i+1}^T)},
\end{equation}
and we use that for the computations because it is positive semidefinite exactly when the original matrix is.
By Lemma~\ref{lemma:bernstein_socp} and Fact~\ref{fact:2x2tonxn}, $\pmat{m_i B_{i-1}^k \mathbf{1}_n& \frac{1}{\sqrt{2}}B_i^k \mathbf{1}_n\\ \frac{1}{\sqrt{2}}B_i^k\mathbf{1}_n & B_{i+1}^k\mathbf{1}_n} \succeq 0$. Let $H_i$ be the Hadamard product between the $i$th matrix and \eqref{eqn:general_deg_matrix_pmp}. Sum $H_i$ over $1 \leq i \leq k-1$ to get 
\begin{equation}
\pmat{\sum_{i=0}^{k-2} w_k(P_i - C_i - C_i^T) B_i^k & \sum_{i=1}^{k-1} C_i B_i^k \\ \sum_{i=1}^{k-1} C_i^T B_i^k & \sum_{i=2}^{k} w_k(P_i - C_i - C_i^T) B_i^k}\succeq 0.
\end{equation}Finally by Lemma~\ref{lem:sumpsdblock}, the sum of the blocks is positive semidefinite. The terms occuring twice have $w_i = \frac{1}{2}$ and the others have $w_i = 1$. Therefore the sum is exactly $P$, which is then positive semidefinite.
\end{proof}
\arbitrarygeneralinclusions*
\begin{proof}[Proof of Theorem~\ref{thm:arbitrary_general_inclusions}]
First we suppose that $p \in \mathcal{NB}_n$. Since $P_i \
succeq 0$, it is bigger than any negative semidefinite matrix, in particular the geometric mean of $P_{i-1}$ and $P_{i+1}$. Therefore $p \in \mathcal{GB}_n$. 

Next we argue that if $p \in \mathcal{GB}_n$ then $C_i = -\sqrt{\frac{w_{i-1}w_{i+1}}{2m_i}}((P_{i-1})_+\#(P_{i+1})_+)$ is feasible for \eqref{eqn:general_deg_matrix_pmp} (or more precisely the congruent matrix \eqref{eqn:matrix_congruence_sufficient}). If either $P_{i-1}$ or $P_{i+1}$ is indefinite, then the only thing to check is that both $P_{i-1} - C_{i-1} - C_{i-1}^T$ and $P_{i+1} - C_{i+1} - C_{i+1}^T$ are positive semidefinite (because the off-diagonal entries are 0). This is exactly the condition that $p \in \mathcal{GB}$. On the other hand, if both are positive semidefinite, then we need to show
\begin{equation}\label{eqn:GBdecomp}
\pmat{\frac{w_{i-1}}{m_i}(P_{i-1})  & \sqrt{2}C_i \\ \sqrt{2}C_i^T & w_{i+1}(P_{i+1})} + \pmat{\frac{w_{i-1}}{m_i}(- C_{i-1} - C_{i-1}^T)  & 0 \\ 0 & w_{i+1}(- C_{i+1} - C_{i+1}^T)} \succeq 0.
\end{equation} 
By Fact~\ref{fact:key-geom-mean}, \begin{equation} \pmat{\frac{w_{i-1}}{m_i}(P_{i-1})  & -\sqrt{2}C_i \\ -\sqrt{2}C_i^T & w_{i+1}(P_{i+1})}
\end{equation} is positive semidefinite. This means for all $x, y$, 
\begin{equation}
0 \leq \pmat{x \\y}^T\pmat{\frac{w_{i-1}}{m_i}(P_{i-1})  & -\sqrt{2}C_i \\ -\sqrt{2}C_i^T & w_{i+1} (P_{i+1})}\pmat{x \\y} = \pmat{x \\-y}^T\pmat{\frac{w_{i-1}}{m_i}(P_{i-1})  & \sqrt{2}C_i \\ \sqrt{2}C_i^T & w_{i+1} (P_{i+1})}\pmat{x \\-y}
\end{equation}
Therefore the first matrix in \eqref{eqn:GBdecomp} is positive semidefinite. The second matrix is positive semidefinite because the block diagonals are geometric means, which are positive semidefinite. Therefore the sum is as well. Hence whenever $p \in \mathcal{GB}_n$, we have $p \in \mathcal{P}_n$. 
\end{proof}
